# Supplementary material for: GraphSnapShot: Caching Local Structure for Fast Graph Learning
Source: arXiv:2406.17918 source file (2025-01-11)
Supplement: Supplementary file 1 [file appendix_u.tex]

\section{Appendix}
\subsection{dgl Experiments}

\subsubsection{datasets}

\begin{table}[H]
\centering
\caption{Overview of OGBN Datasets}
\begin{tabular}{|c|c|c|c|}
\hline
\textbf{Feature} & \textbf{ARXIV} & \textbf{PRODUCTS} & \textbf{MAG} \\ \hline
Type & Citation Net. & Product Net. & Acad. Graph \\ \hline
Nodes & 17,735 & 24,019 & 132,534 \\ \hline
Edges & 116,624 & 123,006 & 1,116,428 \\ \hline
Dim & 128 & 100 & 50 \\ \hline
Classes & 40 & 89 & 112 \\ \hline
Train Nodes & 9,500 & 12,000 & 41,351 \\ \hline
Val. Nodes & 3,500 & 2,000 & 10,000 \\ \hline
Test Nodes & 4,735 & 10,019 & 80,183 \\ \hline
Task & Node Class. & Node Class. & Node Class. \\ \hline
\end{tabular}
\end{table}

\subsubsection{Training Time Acceleration}
This table provides a comparison of the training times (``training time'') of different computational methods (FBL, FCR, FCR-shared cache, OTF, OTF-shared cache) across three settings (\texttt{[20, 20, 20]}, \texttt{[10, 10, 10]}, and \texttt{[5, 5, 5]}). It also calculates the time acceleration percentage relative to FBL for methods other than FBL, expressed as a percentage.

\begin{table}[H]
\centering
\caption{Training Time Acceleration Through Each Method}
\label{tab:training_time_acceleration}
\begin{tabular}{|l|l|c|c|}
\hline
\textbf{Method} & \textbf{Setting} & \textbf{Time (s)} & \textbf{Acceleration (\%)} \\
\hline
FBL             & [20, 20, 20]     & 0.2766                     & -                               \\
                & [10, 10, 10]     & 0.0747                     & -                               \\
                & [5, 5, 5]        & 0.0189                     & -                               \\
\hline
FCR             & [20, 20, 20]     & 0.2571                     & 7.05                            \\
                & [10, 10, 10]     & 0.0639                     & 14.48                           \\
                & [5, 5, 5]        & 0.0163                     & 13.76                           \\
\hline
FCR-shared cache& [20, 20, 20]     & 0.2554                     & 7.69                            \\
                & [10, 10, 10]     & 0.0640                     & 14.33                           \\
                & [5, 5, 5]        & 0.0161                     & 14.76                           \\
\hline
OTF             & [20, 20, 20]     & 0.2460                     & 11.07                           \\
                & [10, 10, 10]     & 0.0568                     & 23.96                           \\
                & [5, 5, 5]        & 0.0145                     & 23.28                           \\
\hline
OTF-shared cache& [20, 20, 20]     & 0.2393                     & 13.49                           \\
                & [10, 10, 10]     & 0.0559                     & 25.23                           \\
                & [5, 5, 5]        & 0.0133                     & 29.63                           \\
\hline
\end{tabular}
\end{table}

\begin{table}[H]
\centering
\caption{Detailed Settings for Each Computational Method}
\label{tab:method_settings}
\begin{tabular}{|l|l|}
\hline
\textbf{Method} & \textbf{Detailed Settings} \\
\hline
FCR & [20, 20, 20], alpha=2, T=50 \\
    & [10, 10, 10], alpha=2, T=50 \\
    & [5, 5, 5], alpha=2, T=50 \\
\hline
FCR-shared cache & [20, 20, 20], alpha=2, T=50 \\
                 & [10, 10, 10], alpha=2, T=50 \\
                 & [5, 5, 5], alpha=2, T=50 \\
\hline
OTF & [20, 20, 20], amp\_rate=2, refresh\_rate=0.15, T=50 \\
    & [10, 10, 10], amp\_rate=2, refresh\_rate=0.15, T=50 \\
    & [5, 5, 5], amp\_rate=2, refresh\_rate=0.15, T=50 \\
\hline
OTF-shared cache & [20, 20, 20], amp\_rate=2, refresh\_rate=0.15, T=50 \\
                 & [10, 10, 10], amp\_rate=2, refresh\_rate=0.15, T=50 \\
                 & [5, 5, 5], amp\_rate=2, refresh\_rate=0.15, T=50 \\
\hline
\end{tabular}
\end{table}

\begin{itemize}
    \item \textbf{OTF-shared cache} shows the highest time acceleration at the smallest setting (\texttt{[5, 5, 5]}), with a \textbf{29.63\% improvement}, highlighting its efficiency for smaller datasets.
    \item Both \textbf{FCR} and \textbf{FCR-shared cache} methods consistently perform better than FBL, especially in medium and smaller settings, indicating significant improvements in training time.
    \item The time acceleration percentages are notably higher in the smallest setting for all methods, suggesting that these optimized approaches are particularly effective for smaller datasets.
\end{itemize}

\subsubsection{Runtime Memory Reduction}
\begin{table}[H]
\centering
\caption{Comparison of Runtime Memory Reduction Across Computational Methods. RM stands for Runtime Memory, ar for amp\_rate/alpha, and rr for refresh\_rate.}
\label{tab:runtime_memory_reduction}
\begin{tabular}{|p{2cm}|p{3.5cm}|c|c|}
\hline
\textbf{Method} & \textbf{Setting} & \textbf{RM (MB)} & \textbf{Reduction (\%)} \\
\hline
FBL & [20]*3 & 6.33 & 0.00\% \\
    & [10]*3 & 4.70 & 0.00\% \\
    & [5]*3    & 4.59 & 0.00\% \\
\hline
FCR & [20]*3, ar=2, T=50 & 2.69 & 57.46\% \\
    & [10]*3, ar=2, T=50 & 2.11 & 55.04\% \\
    & [5]*3, ar=2, T=50    & 1.29 & 71.89\% \\
\hline
FCR-SC & [20]*3, ar=2, T=50 & 4.42 & 30.13\% \\
                 & [10]*3, ar=2, T=50 & 2.62 & 44.15\% \\
                 & [5]*3, ar=2, T=50    & 1.66 & 63.79\% \\
\hline
OTF & [20]*3, ar=2, rr=0.15, T=358 & 4.13 & 34.80\% \\
    & [20]*3, ar=2, rr=0.15, T=50  & 4.19 & 33.86\% \\
    & [10]*3, ar=2, rr=0.15, T=50  & 1.87 & 60.07\% \\
    & [5]*3, ar=2, rr=0.15, T=50     & 0.32 & 93.02\% \\
\hline
OTF-SC & [20]*3, ar=2, rr=0.15, T=50 & 1.41 & 77.68\% \\
                 & [10]*3, ar=2, rr=0.15, T=50 & 0.86 & 81.58\% \\
                 & [5]*3, ar=2, rr=0.15, T=50    & 0.67 & 85.29\% \\
\hline
\end{tabular}
\end{table}

The reduction percentage is calculated by comparing the runtime memory usage of a method under a specific setting to the baseline method's usage at the same setting. The formula used to compute the reduction is given by:
\[
\text{Reduction (\%)} = \left(\frac{\text{Base RM} - \text{Current RM}}{\text{Base RM}}\right) \times 100\%
\]
where:
\begin{itemize}
    \item \textbf{Base RM} represents the runtime memory (in MB) of the baseline method for a given setting, which is the FBL method in this case.
    \item \textbf{Current RM} represents the runtime memory of the current method under the same setting.
\end{itemize}

\begin{itemize}
    \item \textbf{Baseline Setting (FBL)}: All calculations are compared against the FBL method as the baseline, where the reduction is always 0\% because it is compared against itself.
    
    \item \textbf{FCR Method}: 
    \begin{itemize}
        \item For the setting [20, 20, 20], memory reduction is 57.46\%, showing significant effectiveness of this method at larger settings.
        \item For the settings [10, 10, 10] and [5, 5, 5], memory reductions are 55.04\% and 71.89\% respectively, indicating effective memory reduction across various settings, especially at smaller scales.
    \end{itemize}
    
    \item \textbf{FCR-shared cache Method}: 
    \begin{itemize}
        \item This method typically uses more memory than FCR in a shared cache situation but still shows significant memory reductions, especially in the setting [5, 5, 5], with a reduction of 63.79\%.
    \end{itemize}
    
    \item \textbf{OTF Method}: 
    \begin{itemize}
        \item For the setting [20, 20, 20], whether at a longer cycle (T=358) or a shorter cycle (T=50), memory reductions are around 34\%, indicating that the change in response time does not significantly affect memory reduction.
        \item At smaller settings ([5, 5, 5]), memory is reduced by up to 93.02\%, showing extremely high efficiency of the OTF method in handling small-scale tasks.
    \end{itemize}
    
    \item \textbf{OTF-shared cache Method}: 
    \begin{itemize}
        \item This method shows very high memory reduction rates across all settings, particularly in [5, 5, 5] with a reduction of 85.29\%, and 77.68\% in [20, 20, 20], indicating that shared caching significantly enhances memory efficiency in the OTF method.
    \end{itemize}
\end{itemize}

\subsubsection{GPU Usage Reduction}

% given example of amplication rate = 1.5, it means if I want to sample a fanout=10, then I need to first sample 15 as a subgraph.

% For this code, we will move the threshold, and test the GPU usage.

% The GPU usage is computed by sparse graph+ resampled static subgraph, where sparse graph contains those nodes with degree lower than threshold, and the dense graph contains those nodes with degree higher or equal to threshold, and then we need to resampled the dense subgraph by amplified fanout for a cached dense subgraph to GPU, and those sparse graph structure are directly to GPU. The GPU size is computed by total edges storage. 

% Please give out the table for GPU usage comparison on different datasets, compare the influced by amp\_rate and threshold

% dataset, Threshold, Resample amplication Fanout --> GPU Usage (sparse graph+dense graph)

\begin{table}[H]
\centering
\caption{GPU Usage for \texttt{ogbn-arxiv} (edges)}
\label{tab:gpu_usage_arxiv}
\begin{tabular}{cccc}
\hline
\textbf{Threshold} & \textbf{Sparse Graph} & \textbf{Resampled Graph} & \textbf{Total Storage} \\ \hline
10                        & 86,053                        & 948,495                              & 1,034,548              \\
20                        & 223,031                       & 431,520                              & 654,551                \\
30                        & 333,599                       & 223,305                              & 556,904                \\
40                        & 423,513                       & 128,715                              & 552,228                \\
50                        & 491,462                       & 85,125                               & 576,587                \\
60                        & 543,682                       & 62,415                               & 606,097                \\
70                        & 585,752                       & 48,810                               & 634,562                \\
80                        & 619,468                       & 39,855                               & 659,323                \\
90                        & 649,094                       & 33,255                               & 682,349                \\
100                       & 674,965                       & 28,290                               & 703,255                \\
110                       & 698,646                       & 24,225                               & 722,871                \\
120                       & 720,183                       & 20,940                               & 741,123                \\
130                       & 738,536                       & 18,420                               & 756,956                \\
140                       & 755,044                       & 16,335                               & 771,379                \\ \hline
\end{tabular}
\end{table}

\begin{table}[H]
\centering
\caption{GPU Usage Simulation for \texttt{ogbn-products} (edges)}
\label{tab:gpu_usage_products}
\begin{tabular}{cccc}
\hline
\textbf{Threshold} & \textbf{Sparse Graph} & \textbf{Resampled Graph} & \textbf{Total Storage} \\ \hline
10                        & 92,784                        & 30,942,345                           & 31,035,129             \\
20                        & 491,202                       & 26,278,605                           & 26,769,807             \\
30                        & 1,122,314                     & 23,034,195                           & 24,156,509             \\
40                        & 1,894,456                     & 20,644,980                           & 22,539,436             \\
50                        & 2,781,440                     & 18,723,690                           & 21,505,130             \\
60                        & 3,797,306                     & 17,072,610                           & 20,869,916             \\
70                        & 4,943,892                     & 15,588,690                           & 20,532,582             \\
80                        & 6,230,698                     & 14,219,115                           & 20,449,813             \\
90                        & 7,697,986                     & 12,920,310                           & 20,618,296             \\
100                       & 9,327,842                     & 11,708,340                           & 21,036,182             \\
110                       & 11,063,622                    & 10,622,880                           & 21,686,502             \\
120                       & 12,882,860                    & 9,671,610                            & 22,554,470             \\
130                       & 14,737,002                    & 8,839,755                            & 23,576,757             \\
140                       & 16,667,254                    & 8,088,615                            & 24,755,869             \\ \hline
\end{tabular}
\end{table}

\begin{table}[H]
\centering
\caption{GPU Usage Simulationfor \texttt{ogbn-mag} (edges)}
\label{tab:gpu_usage}
\begin{tabular}{cccc}
\hline
\textbf{Threshold} & \textbf{Sparse Graph} & \textbf{Resampled Graph} & \textbf{Total Storage} \\ \hline
10                        & 432,912                       & 4,934,910                           & 5,367,822              \\
20                        & 1,335,788                     & 2,321,400                           & 3,657,188              \\
30                        & 2,059,531                     & 1,307,445                           & 3,366,976              \\
40                        & 2,610,841                     & 813,090                             & 3,423,931              \\
50                        & 3,055,313                     & 533,295                             & 3,588,608              \\
60                        & 3,422,953                     & 363,120                             & 3,786,073              \\
70                        & 3,717,725                     & 257,385                             & 3,975,110              \\
80                        & 3,962,156                     & 187,365                             & 4,149,521              \\
90                        & 4,159,659                     & 140,670                             & 4,300,329              \\
100                       & 4,322,855                     & 107,835                             & 4,430,690              \\ \hline
\end{tabular}
\end{table}

% Baseline with NeighborSampler in dgl.

% Test FCR, OTF (,)x(,) experiments settings.

% memory reduction, acc acceleration comparison

% Setting - Time - Mem table for reduction

% For ogbn-products
% Setting (FCR, OTF) - Time reduction - Mem table
% Comparison: T, T_refresh, T_fetch, refresh_rate, fetch_rate, amp_rate 

% **time reduction** and **memory** figures

% For ogbn-arxiv
% Comparison: T, T_refresh, T_fetch, refresh_rate, fetch_rate
% Setting (FCR, OTF) - Time reduction - Mem table

% For ogbn-mag
% Comparison: T, T_refresh, T_fetch, refresh_rate, fetch_rate

% \subsubsection{** Accuracy Ablation}
% Accuracy ablation for different setting (N*N matrix\）

% OK

\subsection{PyTorch Experiments}
\begin{table}[H]
\centering
\begin{tabular}{|l|r|r|r|r|}
\hline
\textbf{Dataset} & \textbf{Nodes} & \textbf{Edges} & \textbf{Features} & \textbf{Classes} \\ \hline
PubMed           & 19,717         & 44,338         & 500               & 3                \\ \hline
Cora             & 2,708          & 5,429          & 1,433             & 7                \\ \hline
CiteSeer         & 3,312          & 4,732          & 3,703             & 6                \\ \hline
\end{tabular}
\caption{Comparison of Datasets}
\label{tab:dataset-comparison}
\end{table}

\begin{table}[H]
\centering
\begin{tabular}{|c|c|c|}
\hline
\textbf{Operation}           & \textbf{Duration (s)} & \textbf{Simulation Frequency} \\ \hline
Simulated Disk Read          & 5.0011                      & 0.05                               \\ \hline
Simulated Disk Write         & 1.0045                      & 0.05                               \\ \hline
Simulated Cache Access      & 0.0146                      & 0.05                               \\ \hline
In-Memory Computation & Real Computation                      & Real Computation                               \\ \hline
\end{tabular}
\caption{Simulation Durations and Frequencies}
\label{tab:simulation-duration-access}
\end{table}

\begin{table}[H]
\centering
\begin{tabular}{|l|c|c|c|}
\hline
\textbf{Operation}           & \textbf{k\_h\_sampling} & \textbf{k\_hop\_retrieval} & \textbf{k\_h\_resampling} \\ \hline
Disk Read          & $\checkmark$                         &                           & $\checkmark$                           \\ \hline
Disk Write         & $\checkmark$                         &                           & $\checkmark$                           \\ \hline
Memory Access      &                           & $\checkmark$                         &                             \\ \hline
\end{tabular}
\caption{Function Access Patterns for Different Operations}
\label{tab:function-access-patterns}
\end{table}

\begin{table}[H]
\centering
\caption{Experimental Settings - Setting 1}
\label{tab:experimental-settings-setting-1}
\begin{tabular}{|c|c|c|c|c|}
\hline
\textbf{Dataset} & \textbf{Alpha} & \textbf{Presampled} & \textbf{Resampled} & \textbf{Sampled Depth} \\ \hline
CiteSeer         & 0.1, ..., 0.9 & 100 & 40 & 1, 2, 3, 4 \\ \hline
Cora             & 0.1, ..., 0.9 & 100 & 40 & 1, 2, 3, 4 \\ \hline
PubMed           & 0.1, ..., 0.9 & 100 & 40 & 1, 2, 3, 4 \\ \hline
\end{tabular}
\vspace{5pt} % Adjust the space here as needed
\end{table}

\begin{table}[H]
\centering
\caption{Experimental Settings - Setting 2}
\label{tab:experimental-settings-setting-2}
\begin{tabular}{|c|c|c|c|c|}
\hline
\textbf{Dataset} & \textbf{Alpha} & \textbf{Presampled} & \textbf{Resampled} & \textbf{Sampled Depth} \\ \hline
CiteSeer         & 0.1, ..., 0.9 & 20 & 10 & 1, 2, 3, 4 \\ \hline
Cora             & 0.1, ..., 0.9 & 20 & 10 & 1, 2, 3, 4 \\ \hline
PubMed           & 0.1, ..., 0.9 & 20 & 10 & 1, 2, 3, 4 \\ \hline
\end{tabular}
\end{table}

\begin{table}[H]
\centering
\caption{IOCostOptimizer Functionality Overview}
\label{tab:functionality-overview}
\begin{tabular}{|c|p{8cm}|}
\hline
\textbf{Abbreviation} & \textbf{Description} \\
\hline
Adjust & Adjusts read and write costs based on system load. \\
\hline
Estimate & Estimates query cost based on read and write operations. \\
\hline
Optimize & Optimizes query based on context ('high\_load' or 'low\_cost'). \\
\hline
Modify Load & Modifies query for high load optimization. \\
\hline
Modify Cost & Modifies query for cost efficiency optimization. \\
\hline
Log & Logs an I/O operation for analysis. \\
\hline
Get Log & Returns the log of I/O operations. \\
\hline
\end{tabular}
\end{table}

% \begin{table}[H]
% \centering
% \caption{BufferManager Class Methods}
% \label{tab:buffermanager-class-methods}
% \begin{tabular}{|p{4cm}|p{8cm}|}
% \hline
% \textbf{Method} & \textbf{Description} \\
% \hline
% \texttt{\_\_init\_\_(self, capacity)} & Initialize the buffer manager with a specified capacity. \\
% \hline
% \texttt{load\_data(self, key, data)} & Load data into the buffer. \\
% \hline
% \texttt{get\_data(self, key)} & Retrieve data from the buffer. \\
% \hline
% \texttt{store\_data(self, key, data)} & Store data in the buffer. \\
% \hline
% \end{tabular}
% \end{table}

\begin{table}[H]
\centering
\caption{BufferManager Class Methods}
\label{tab:buffermanager-class-methods}
\begin{tabular}{|p{2cm}|p{8cm}|}
\hline
\textbf{Method} & \textbf{Description} \\
\hline
\texttt{init} & Initialize the buffer manager with capacity. \\
\hline
\texttt{load} & Load data into the buffer. \\
\hline
\texttt{get} & Retrieve data from the buffer. \\
\hline
\texttt{store} & Store data in the buffer. \\
\hline
\end{tabular}
\end{table}

% \begin{table}[H]
% \centering
% \caption{BufferManager Class Methods}
% \label{tab:buffermanager-class-methods}
% \begin{tabular}{|l|p|}
% \hline
% \textbf{Method} & \textbf{Description} \\
% \hline
% \texttt{\_\_init\_\_(self, capacity)} & Initialize with specified capacity. \\
% \hline
% \texttt{load\_data(self, key, data)} & Load data into the buffer. \\
% \hline
% \texttt{get\_data(self, key)} & Retrieve data from the buffer. \\
% \hline
% \texttt{store\_data(self, key, data)} & Store data in the buffer. \\
% \hline
% \end{tabular}
% \end{table}
